# Supplementary material for: GPG: A Simple and Strong Reinforcement Learning Baseline for Model Reasoning
Source: arXiv:2504.02546 source file (2026-02-03)
Supplement: Supplementary file 2 [file 15B_loss.tex]

\begin{figure}[t]
\begin{center}
\begin{tabular}{c@{}c@{}c}
\hspace{-5mm}
    \includegraphics[width=0.33\linewidth]{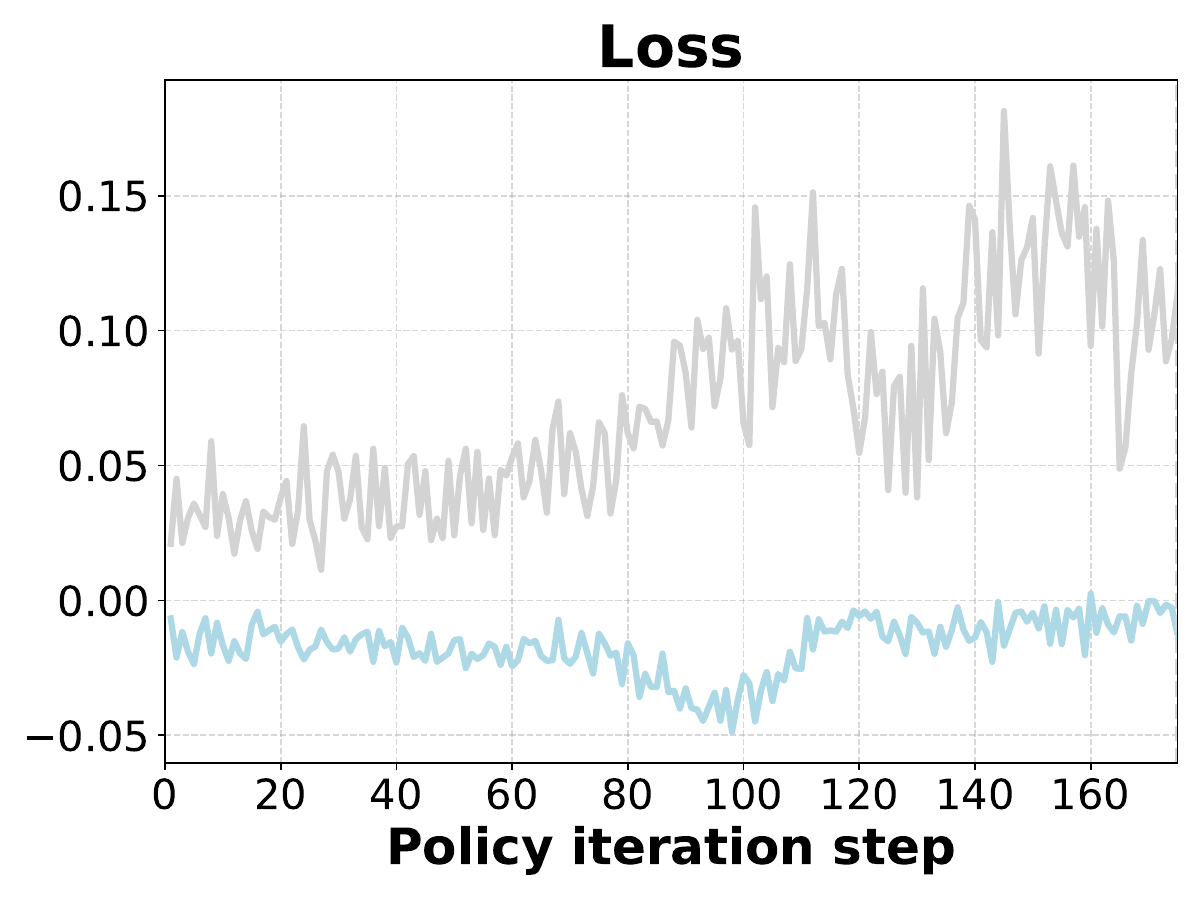} \ &
    \includegraphics[width=0.33\linewidth]{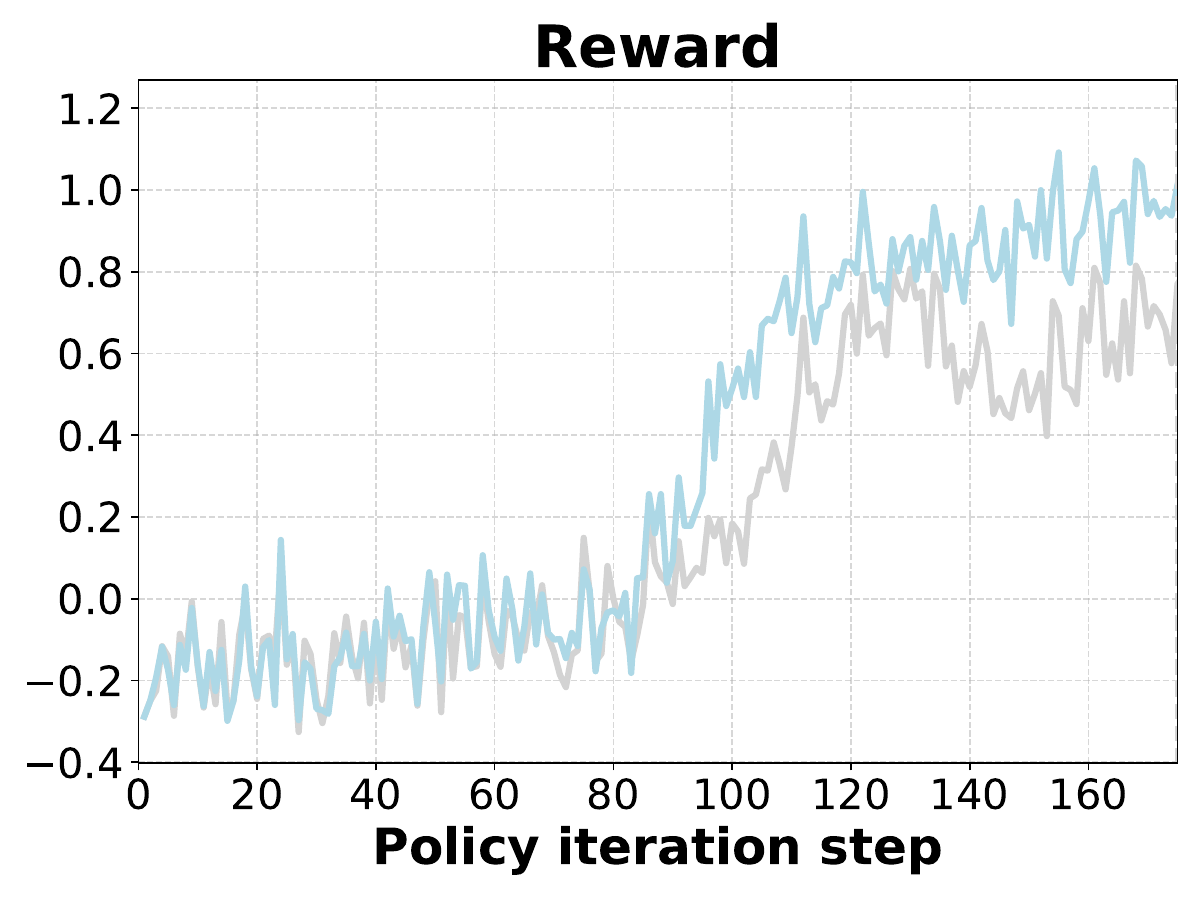} \ &
    \includegraphics[width=0.33\linewidth]{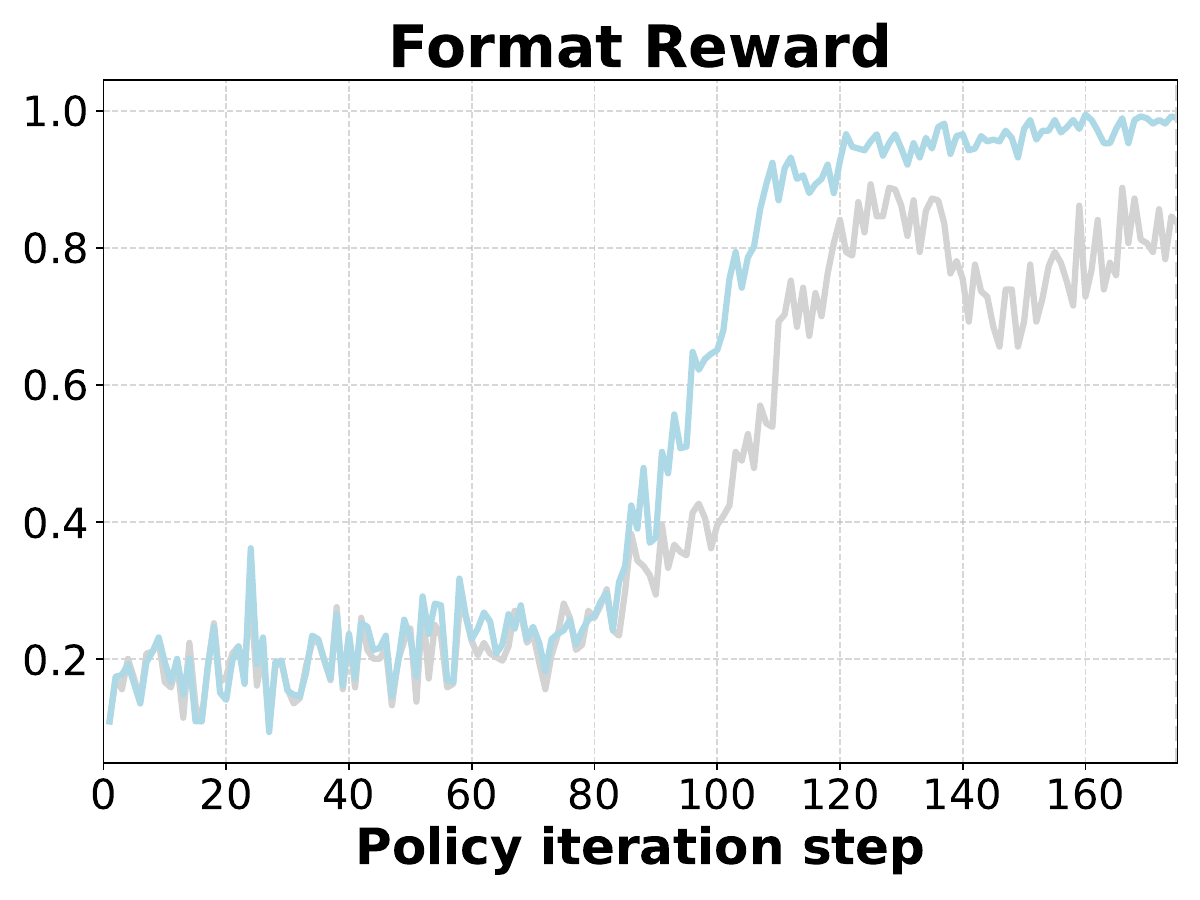} \\
\end{tabular}
\begin{tabular}{c@{}c@{}c}
\hspace{-5mm}
    \includegraphics[width=0.33\linewidth]{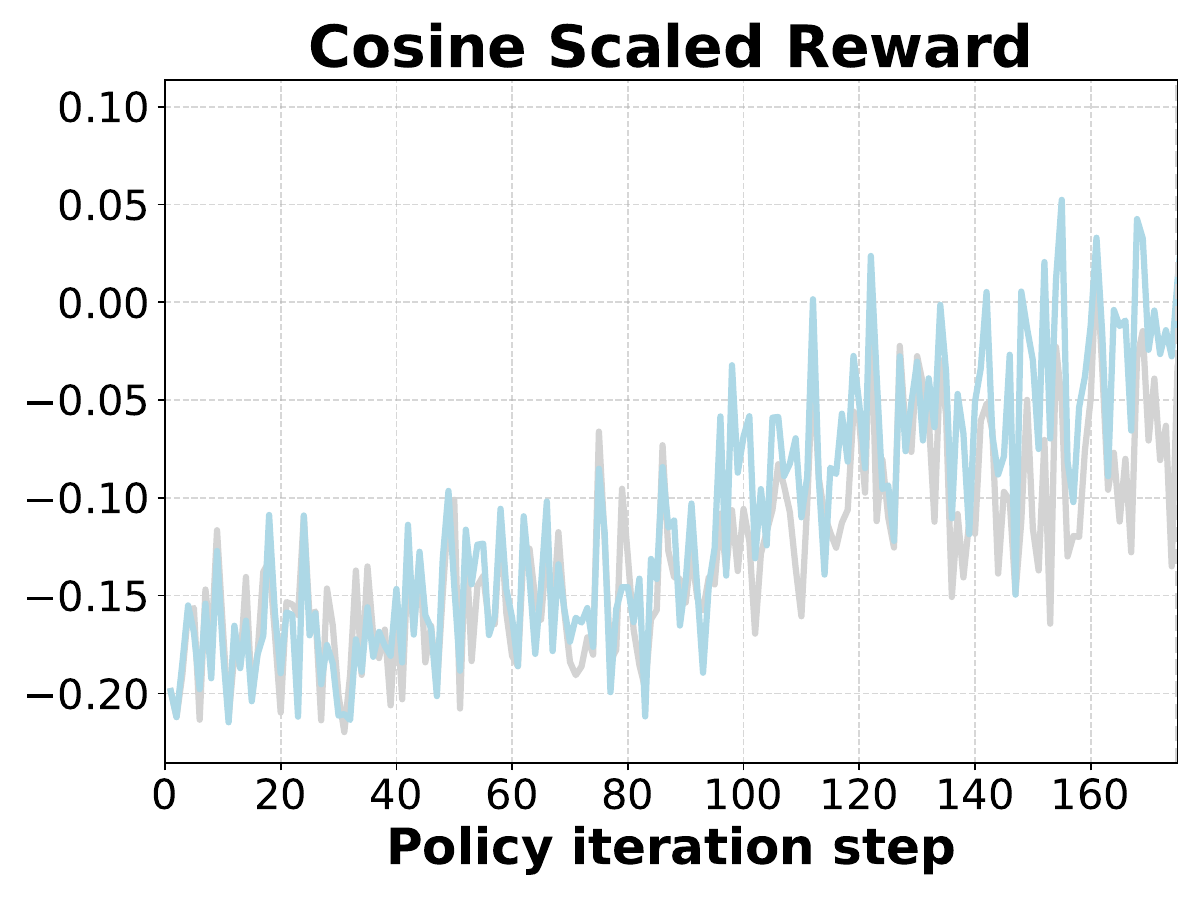} \ &
    \includegraphics[width=0.33\linewidth]{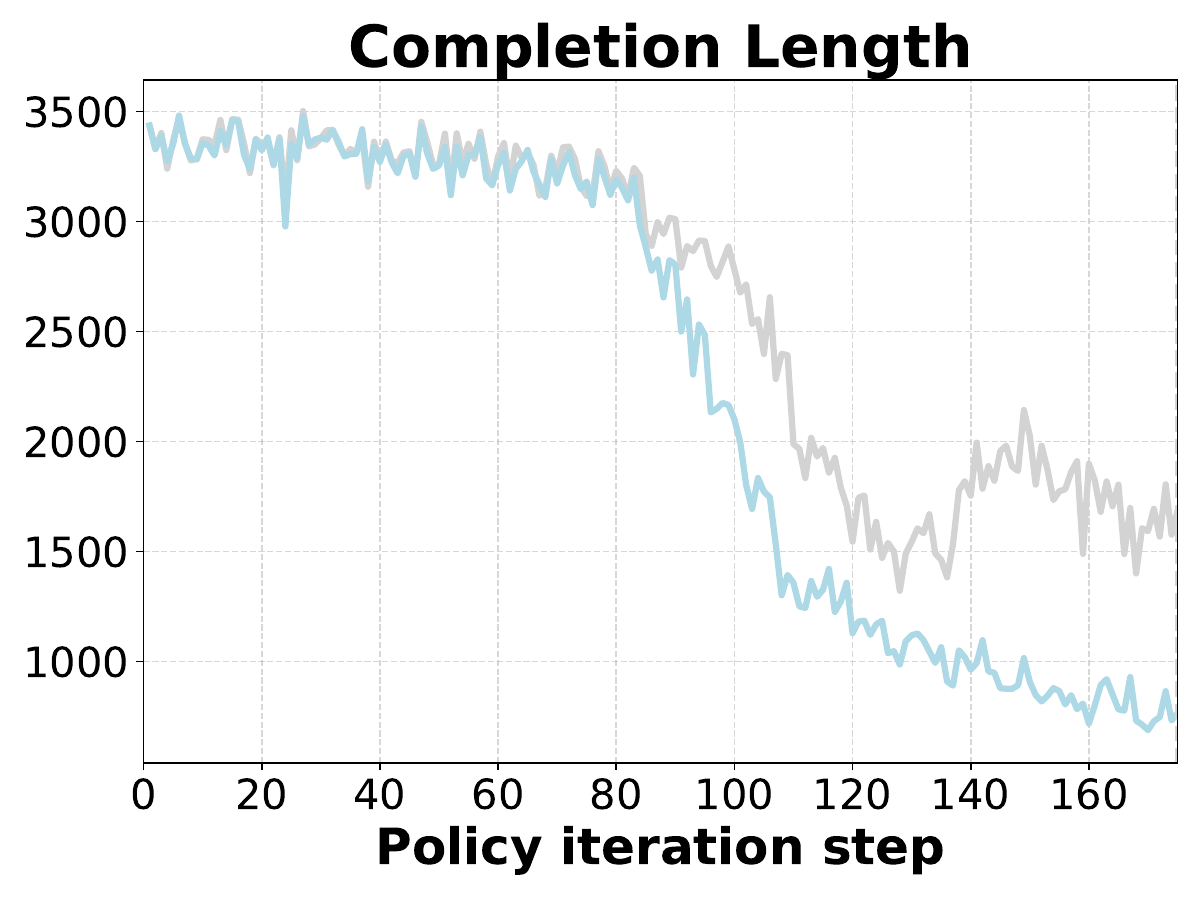} \ &
    \hspace{0mm}
    \raisebox{9mm}{\includegraphics[width=0.35\linewidth]{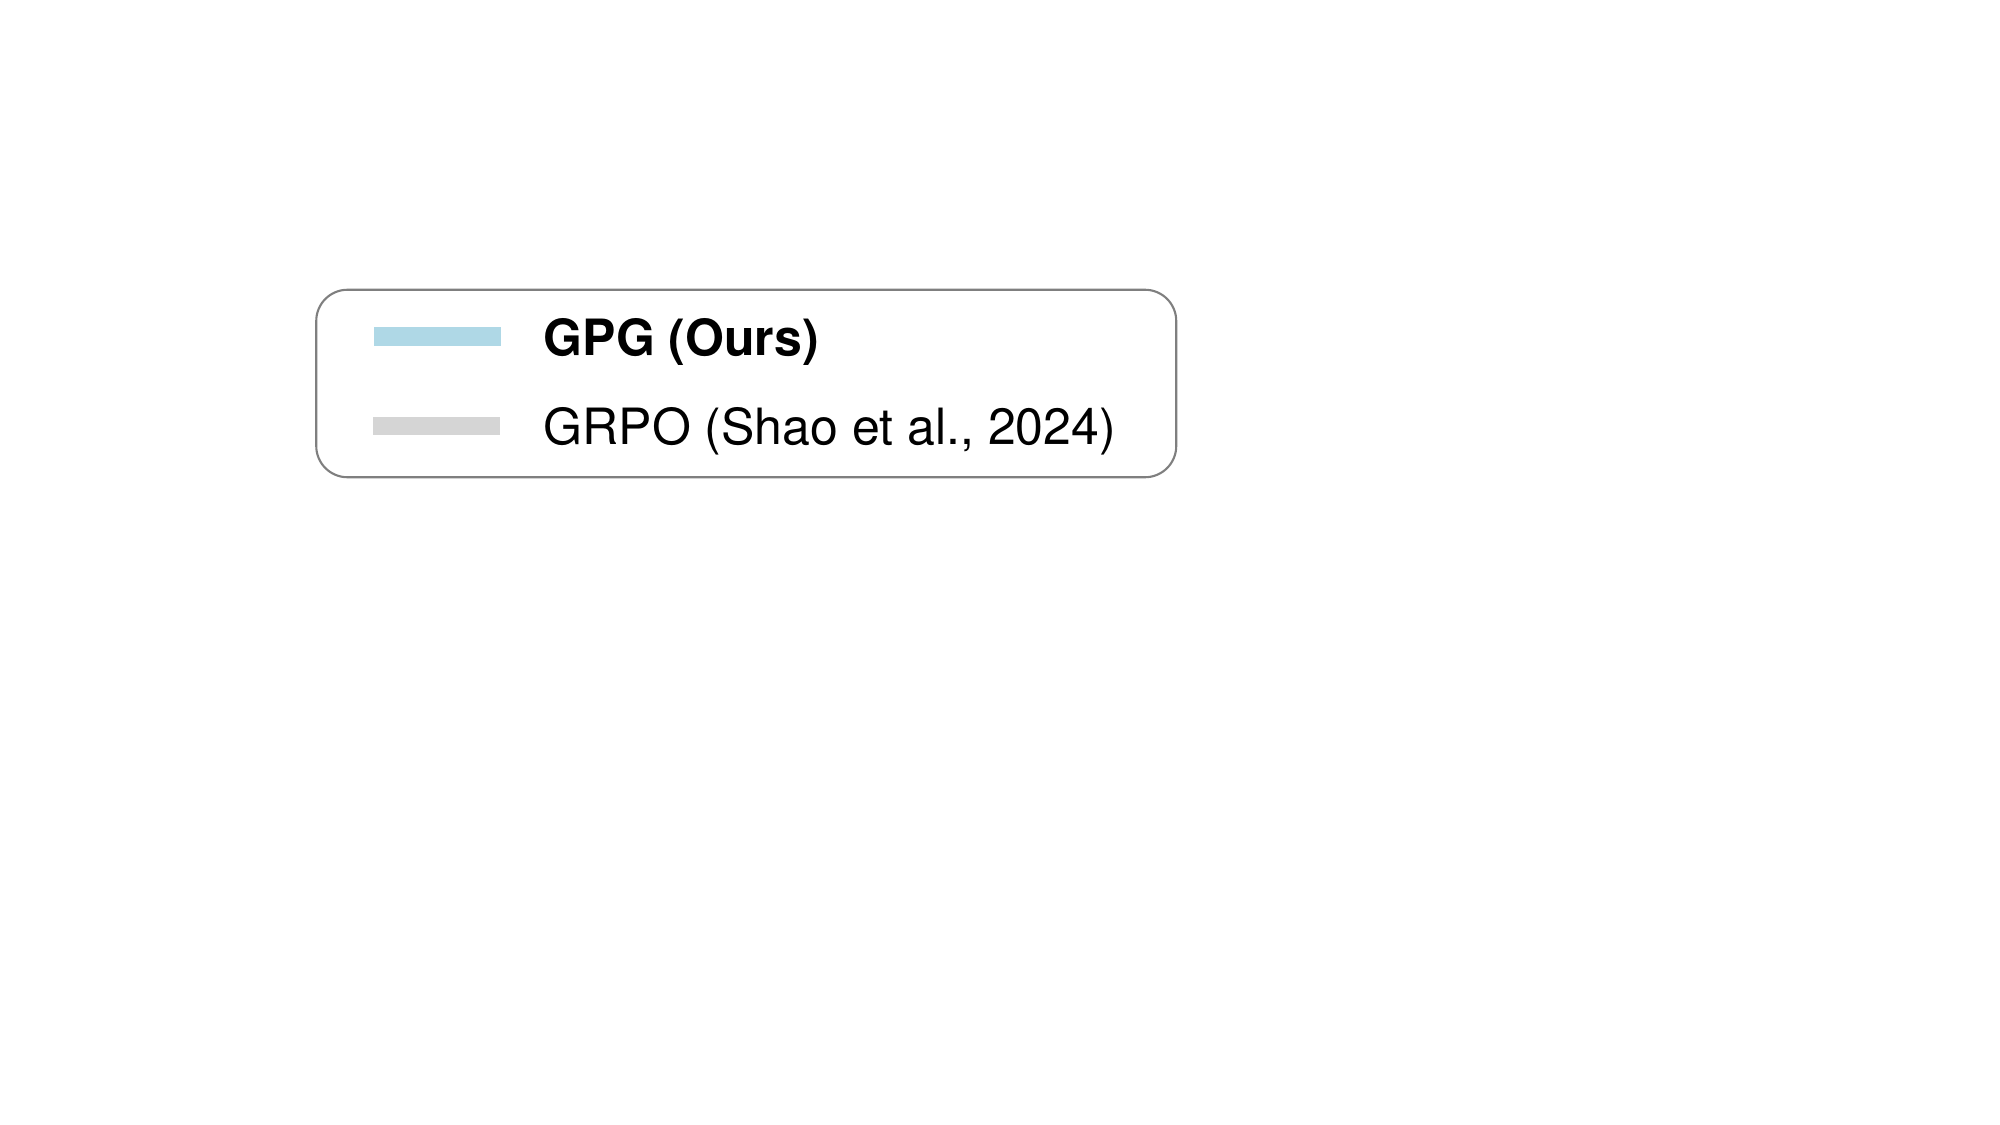}} \\
\end{tabular}
\end{center}
\vspace{-3mm}
\caption{Comparison of GPG and GRPO in terms of training loss, rewards and completion length. The experiments are based on DeepSeek-R1-Distill-Qwen-1.5B as same as Table.~\ref{tab:open-rs}.}
\vspace{-3mm}
\label{fig:training_metrics}
\end{figure}
