# Supplementary material for: GPG: A Simple and Strong Reinforcement Learning Baseline for Model Reasoning
Source: arXiv:2504.02546 source file (2026-02-03)
Supplement: Supplementary file 5 [file Prompt-for-openr1.tex]

\begin{figure*}[ht]
\vspace*{-2.00mm}
\centering
\begin{tcolorbox}[title=System Prompt for  Mathematical Reasoning]
\textbf{Prompt of Open-rs:} A conversation between User and Assistant. The user asks a question, and the Assistant solves it. The assistant first thinks about the reasoning process in the mind and then provides the user with the answer, and put your final answer within boxed\{\}. The reasoning process and answer are enclosed within <think> </think> and <answer> </answer> tags, respectively, i.e., <think> reasoning process here </think> <answer> answer here </answer>. Note that respond by English, NOT use other languages.
\\
\textbf{Prompt of Open-r1:} You are a helpful AI Assistant, designed to provided well-reasoned and detailed responses. You FIRST think about the reasoning process as an internal monologue and then provide the user with the answer. The reasoning process MUST BE enclosed within <think> and </think> tags.
\end{tcolorbox}
\label{tc:Prompt-for-open}
\vspace*{-6.00mm}
\end{figure*}
