# Supplementary material for: GPG: A Simple and Strong Reinforcement Learning Baseline for Model Reasoning
Source: arXiv:2504.02546 source file (2026-02-03)
Supplement: Supplementary file 7 [file gpg_algo.tex]

\begin{algorithm}

	\caption{Group Policy Gradient (GPG)}
	\label{alg:GPG}
	\begin{algorithmic}[1]
		\REQUIRE $o~~[\text{shape: }(B, G, C, dim)] \leftarrow$ Model Output, $r \leftarrow$ Reward, $\beta_{th}$
        \STATE Collecting samples and calculate $\hat{A}$ and $\alpha$ based on Equation~\ref{equ:advantages} and Equation~\ref{eq:alpha} until $\alpha < \frac{1}{\beta_{th}}$ 
        \STATE Calculate $\log\pi_{\theta}(o) [per\_token\_logps]$ based on $o$ and model $\pi_{\theta}$
        \STATE $loss \leftarrow -\log\pi_{\theta}(o) \cdot \hat{A} * \alpha$  
        \ENSURE $loss$
	\end{algorithmic}
\end{algorithm}
\vspace*{-0.4cm}
